# Supplementary material for: Radiance Field Learners As UAV First-Person Viewers
Source: arXiv:2408.05533 source file (2024-08-10)
Supplement: Supplementary file 1 [file X_suppl.tex]

\clearpage
\setcounter{page}{1}

\title{Supplementary Material for Radiance Field Learners As UAV First-Person Viewers} 
\maketitle

% \appendix

\setcounter{section}{0} 

\setcounter{figure}{0} 

\setcounter{table}{0}  

\section{Overview}
In this document we provide more details of our approach, additional methodology and experimental results and analysis, and further discussions. It is organized as follows:
\begin{itemize}
    \item \S \ref{sec:add_preliminary}: More details in \textbf{Preliminary}.
    \item \S \ref{sec:add_camera_space}: More details about \textbf{Camera Space Warping}.
    \item \S \ref{sec:add_dataset}: More details about our \textbf{UAV Dataset Collection}.
    \item  \S \ref{sec:add_implementation}: More details about \textbf{Implementation Details}.
    \item \S \ref{sec:add_exp}: More \textbf{Experimental Results}.
\end{itemize}

\section{Preliminary}
\label{sec:add_preliminary}
Previous NeRF \cite{mildenhall2021nerf,yu2021pixelnerf,chen2021mvsnerf} methods synthesize images by sampling 5D coordinates (location and viewing direction) along camera rays, feeding those locations into an MLP to produce a color and volume density, and using volume rendering techniques to composite these values into an image. We composite the colors of all points $\delta_i$ on a camera ray $\phi$ emitting from a pixel to compute the pixel color $c_{\phi} = (r_{\phi}, g_{\phi}, b_{\phi})$ for Eq.~\ref{eq:color_loss} by:
\begin{equation}
    c_{\phi}=\sum_{\delta_i \in \phi} \left[\prod_{j=0}^{i-1}(1-o_{\delta_j})\right]o_{\delta_i} c_{\delta_i}
\end{equation}
\begin{equation}
    o_{\delta_i} = 1 - e^{-\tau_{\delta_i}d_{\delta_i}}
\end{equation}
where $d_{\delta_i}$ is the density in \S \ref{sec:loss},  and $\tau_{\delta_i}$ is the marching step in the original
space. When sampling points in ray marching, we perform uniform sampling on the warp space, and we get a non-uniform sampling in the original space. We perform a linear approximation let the distance between $\delta_{i+1}$ and $\delta_{i}$ be approxmated by $l=\tau_{\delta_i}||J_{\delta_i}\mathbf{d}||_2$ and get:
\begin{equation}
    \tau_{\delta_i} = \frac{l}{||J_{\delta_i}\mathbf{d}||_2}
\end{equation}
where $J_{\delta_i}$ is the Jacobian matrix at $\delta_i$ from the original space to the warp space. Here $l$ is the
parameter controlling sample density and we empirically set $l=\sqrt{3}$, \textit{i.e.}, the diagonal length of the unit cube in the warp space.

% \begin{figure}[t]
%   \centering
%    \includegraphics[width=1.0\linewidth]{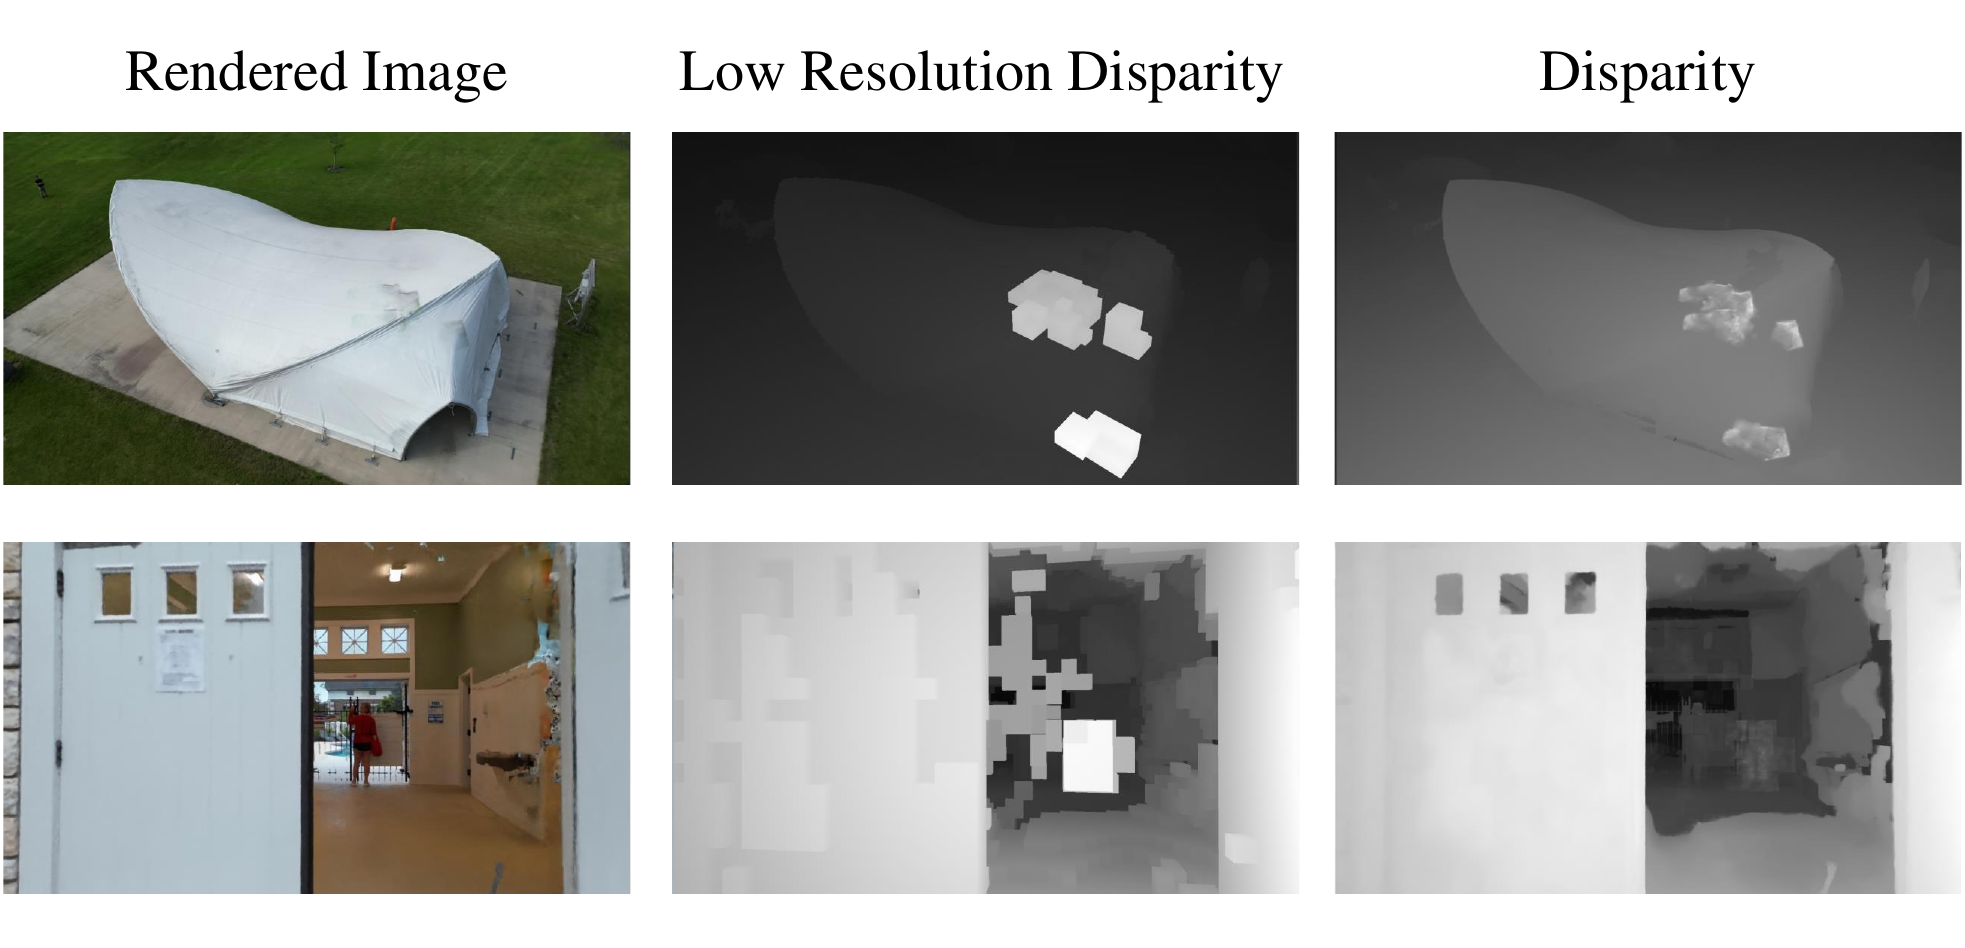}
%    \caption{\textbf{Illustration of disparity alignment.} The absence of local granularity results in a substantial difference in reciprocal depth disparity between two resolutions (see \S \ref{sec:loss}).}
%    \label{fig:more_disparity_loss}
% \end{figure}

\section{Camera Space Warping} 
\label{sec:add_camera_space}
As described in \S \ref{sec:space_estimation}, the camera space is warped with different warping functions in various blocks. In order to render the color $c_{\phi} = (r_{\phi}, g_{\phi}, b_{\phi})$ for the camera ray $\phi$ emitting from a pixel, we first sample points $\delta_i \in \phi$ on this ray. These sampled points are warped by the space warping function $H$ to a new space. Given the region $\Omega$ with the selected cameras, we project the sampled points to the selected cameras, concatenate the projected coordinates, and obtain the high-dimensional coordinates. By eigen decomposition, we obtain the matrix $H'$, which defines the directions of the projection axes, with the first three largest eigenvalues. Let us denote the Jacobian matrix from the original space to the image space as $J_{O \rightarrow I}$ derived from the image projection function, and the Jacobian matrix from the image space to the warp space as $J_{I \rightarrow W} = H = \Omega H'$. Our target is to compute the Jacobian matrix $J_{W \rightarrow I}$ and put a constraint that the maximum value of each column vector of $J_{W \rightarrow I}$ equals 1. Hence, we present the Jacobian matrix $J_{W \rightarrow I}$ from the warp space to  the image space by:
\begin{align}
    J_{W \rightarrow I} &= J_{O \rightarrow I} J_{O \rightarrow W}^{-1} \\
    &= J_{O \rightarrow I} (J_{I \rightarrow W} J_{O \rightarrow I})^{-1} \\
    &= J_{O \rightarrow I} (\Omega H' J_{O \rightarrow I})^{-1} \\
    &= J_{O \rightarrow I} (H' J_{O \rightarrow I})^{-1} \Omega^{-1} 
\end{align}
After block subdivision in \S \ref{sec:space_estimation}, visible cameras aren't directly suitable for space warping as some don't fully cover the region. We propose an effective camera rectification strategy by rotating view directions towards the region's center, ensuring meaningful coordinate warping for most points.

\begin{figure*}[t]
  \centering
   \includegraphics[width=1.0\linewidth]{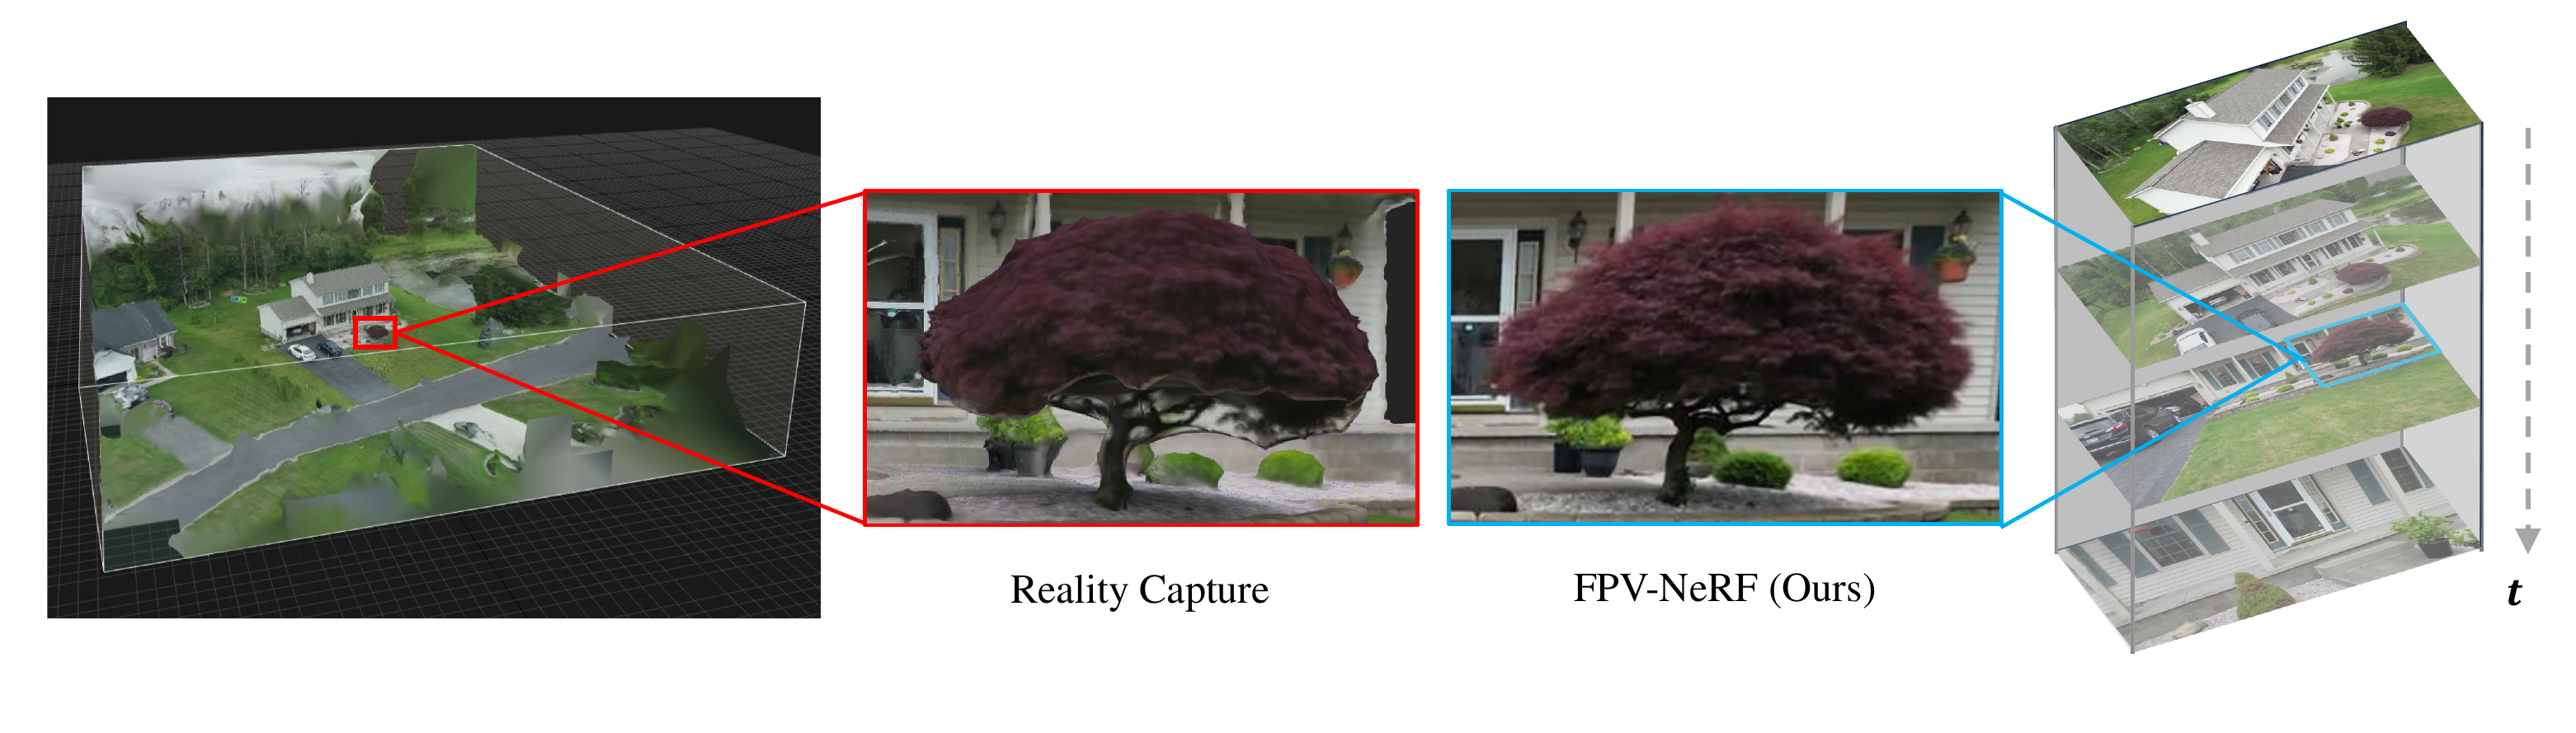}
   \caption{\textbf{Comparison between results from traditional 3D reconstruction (Reality Capture) and FPV-NeRF.} Despite the capability of 3D reconstruction to explicitly generate complete three-dimensional scene models, it often falls short in capturing intricate details. In contrast, our method excels by rendering finer, more realistic details at a higher resolution than conventional 3D reconstruction techniques.}
   \label{fig:comparison_rc}
\end{figure*}

\begin{wrapfigure}{r}{0.61\textwidth}
  \centering
   \includegraphics[width=1.0\linewidth]{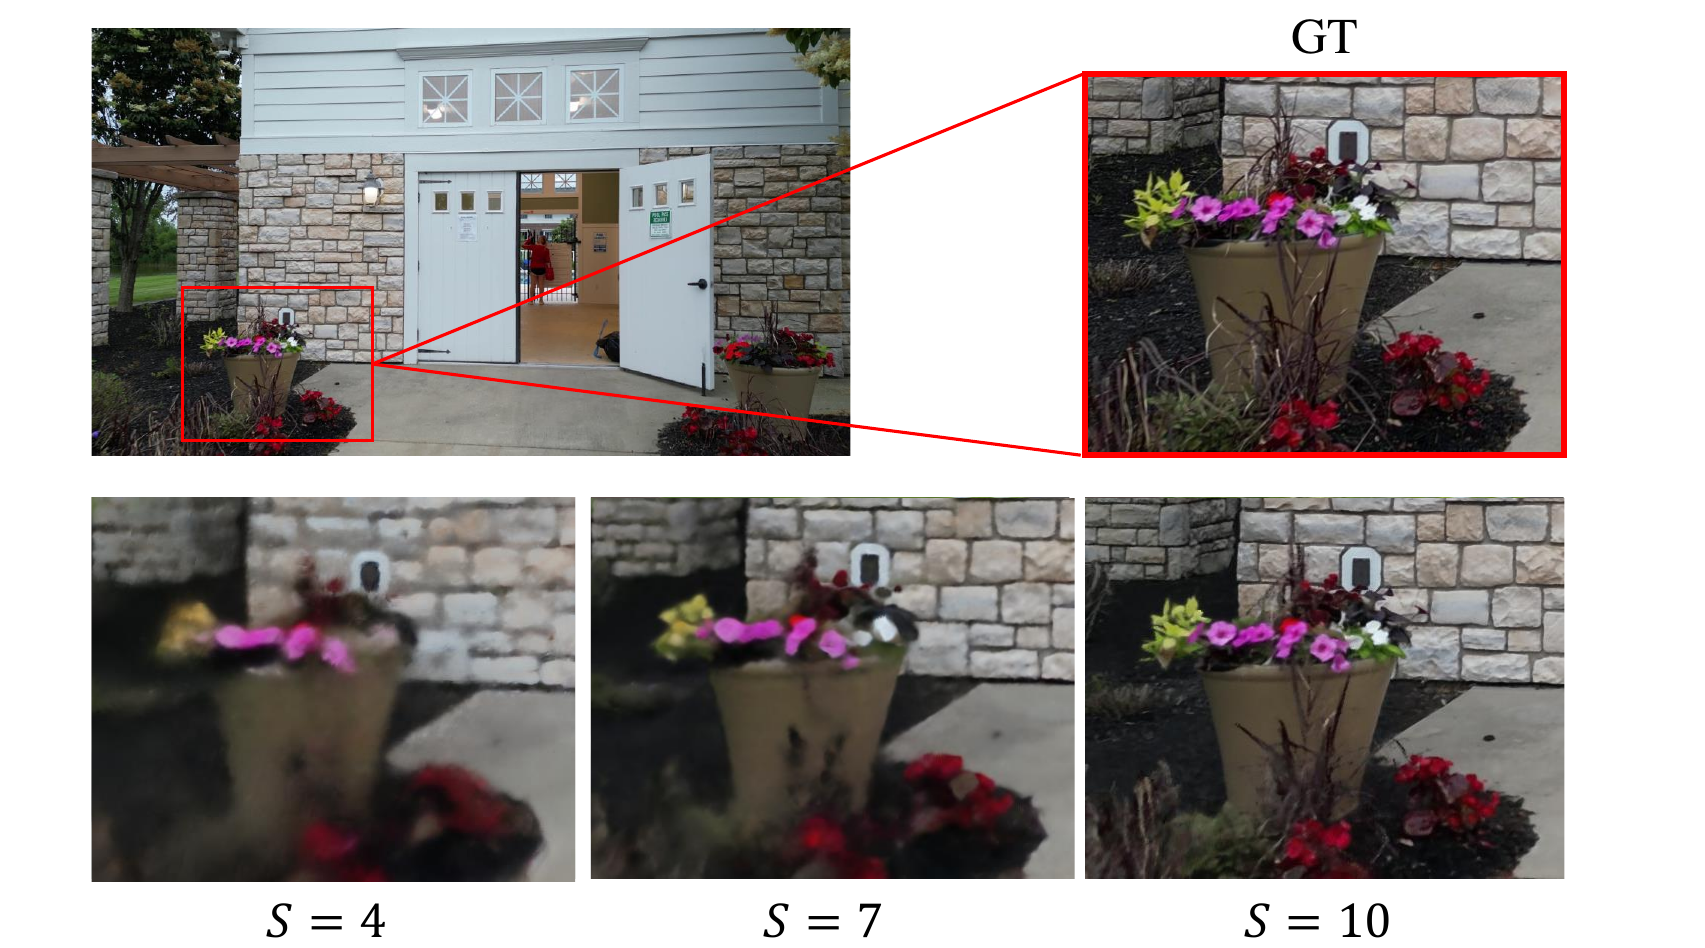}
   \caption{\textbf{More comparison of different point location embedding parameter $S$ in Eq.~\ref{eq:point}.} Larger $S$ exhibits more low-frequency and high-frequency components of the scene (see \S \ref{sec:encoder}).}
   \label{fig:more_point_location}
\end{wrapfigure}

\begin{figure*}[t]
  \centering
   \includegraphics[width=1.0\linewidth]{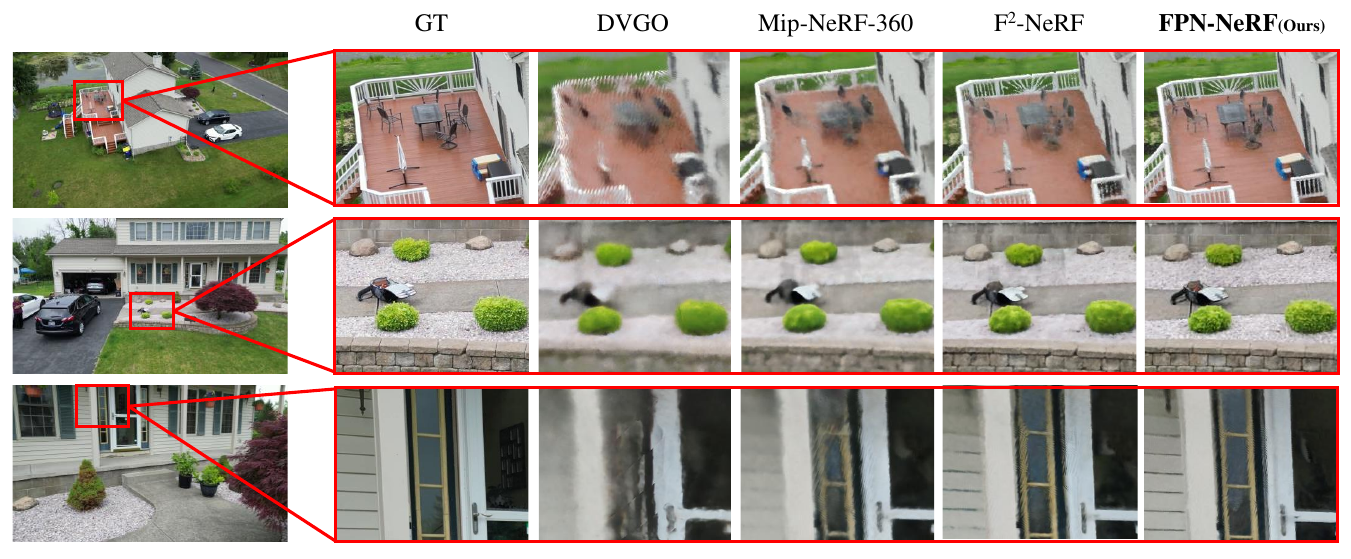}
   \caption{\textbf{More comparison results with SOTA methods.}  On our UAV dataset, each level contains $2^{21}$ feature vectors and are trained for 80k steps. We follow the commonly-adopted settings that set one of every eight images as testing images and the other as the training set.}
   \label{fig:more_comparison_sota}
\end{figure*}

\section{Dataset Collection Details} 
\label{sec:add_dataset}
% In the course of our experimental endeavors, each scenario video is meticulously acquired via the DJI mini3 pro, encompassing a temporal span ranging from 3 to 7 minutes. Simultaneously, the operational altitudes of the UAV manifest a diverse range, extending from 40 to 170 meters. The scenes captured include \textit{market}, \textit{garden}, \textit{park}, \textit{foundation}, \textit{library}, \textit{etc.}, all of which are recorded in New York City, USA.

% In the exposition of our aggregated dataset pertaining to UAV, as elucidated in \S \ref{sec:uav_dataset}, an exhaustive calibration procedure unfolds, probing into both internal and external dimensions. This meticulous endeavor is centered upon the precise determination of intrinsic and extrinsic parameters, firmly grounded in a predetermined image size of $3024 \times 4032$ pixels.

% The scrutiny of camera intrinsics entails a discerning analysis of critical properties, encompassing focal length, principal point, radial distortion, skew, and the intrinsic matrix. The focal length for the UAV camera, a pivotal intrinsic parameter essential for accurately mapping pixel coordinates to real-world spatial dimensions, is computed to be $(2.858 \times 10^3, 2.845 \times 10^3)$ in our experimental investigations. 
The process begins with selecting the appropriate UAV platform equipped with a high-quality camera capable of capturing the required resolution and frame rate. We choose the DJI Mini 3 Pro, as it comes equipped with a smart flight battery that offers an extended maximum flight time of up to 34 minutes. Its 1/1.3-inch image sensor features dual native ISO, supporting straight-out HDR imaging for enhanced dynamic range, preserving details in both bright and dark areas and elevating overall picture depth. Additionally, it supports recording 4K HDR videos and capturing 48-megapixel RAW format photos. Prior to the flight, the research team carefully maps out the flight path, considering factors such as terrain, weather conditions, and any potential obstacles. We also conduct pre-flight checks to ensure compliance with no-fly zones and apply for permits from relevant local government agencies in advance. During the flight, the UAV is operated by a skilled pilot who follows the predetermined route while ensuring smooth and steady camera movements to minimize motion blur and distortion. Additionally, data collection may involve multiple flights to cover the desired area adequately. Once the video footage is captured, it undergoes thorough post-processing, including stabilization, calibration, and data annotation for analysis. The principal point, indicative of the optical epicenter of the camera, undergoes meticulous examination alongside radial distortion, addressing inherent lens imperfections. Skew, quantifying non-orthogonality in image axes, undergoes careful assessment, while the intrinsic matrix amalgamates the collective impact of these parameters. This meticulously calibrated framework forms the cornerstone for a nuanced comprehension of the intricacies inherent in the UAV camera, thereby fortifying the foundation for subsequent applications in the domains of UAV-based imaging and mapping.

\begin{table}
  \begin{minipage}[T]{0.49\linewidth}
  \vspace{-6.5ex}
  \centering
  \caption{\textbf{Impact of the number of block subdivision levels.} We gradually increase the subdivision level numbers by 4 to indicate the effective of block subdivision in \S \ref{sec:space_estimation}.}
  \label{tab:subdivision_level}
  \scalebox{0.72}{
  % \begin{tabular}{@{}lcccc@{}}
  \begin{tabular}{c|c|ccc}
    \hline \thickhline
    \rowcolor{mygray}
    Sub. Levels & Tr. time & PSNR$_\uparrow$ & SSIM$_\uparrow$ & LPIPS$_{\mathrm{(VGG)}\downarrow}$ \\
    \hline \hline
    
    $\leq 4$  & 1.1h & 21.90 & 0.634 & 0.436 \\
    $\leq 8$  & 2.4h & 23.07 & 0.672 & 0.411 \\
    $\leq 12$ & 3.6h & 24.13 & 0.705 & 0.398 \\ 
    $\mathbf{\leq 16}$  & 5.5h & \textbf{26.83} & \textbf{0.769} & \textbf{0.364} \\
    
    \bottomrule
  \end{tabular}
  }
  \vspace{7ex}
  \caption{\textbf{Impact of the number of resolution levels.} We incrementally raise the resolution numbers by 2 to demonstrate the effectiveness of cross-resolution attention in \S \ref{sec:encoder}.}
  \label{tab:resolution_level}
  \scalebox{0.72}{
  % \begin{tabular}{@{}lcccc@{}}
  \begin{tabular}{c|c|ccc}
    \hline \thickhline
    \rowcolor{mygray}
    Res. Levels & Tr. time & PSNR$_\uparrow$ & SSIM$_\uparrow$ & LPIPS$_{\mathrm{(VGG)}\downarrow}$ \\
    \hline \hline
    
    2  & 0.8h & 19.87 & 0.594 & 0.501 \\
    4  & 1.9h & 21.62 & 0.635 & 0.476 \\
    6 & 2.7h & 22.90 & 0.683 & 0.438 \\ 
    8 & 4.3h & 24.21 & 0.719 & 0.402 \\ 
    \textbf{10}  & 5.5h & \textbf{26.83} & \textbf{0.769} & \textbf{0.364} \\
    
    \bottomrule
  \end{tabular}
  }
  \end{minipage}
  \hspace{0.01\linewidth}
  \begin{minipage}[T]{0.49\linewidth}
  \vspace{3ex}
  \centering
  \caption{\textbf{Impact of MLP dimension.} We compare performances with varying MLP dimensions, while keeping the attention layer settings constant, to illustrate the influence of the parameter amount.}
  \label{tab:mlp_dim}
  \scalebox{0.72}{
  % \begin{tabular}{@{}lcccc@{}}
  \begin{tabular}{c|c|ccc}
    \hline \thickhline
    \rowcolor{mygray}
    MLP Dim. & Tr. time & PSNR$_\uparrow$ & SSIM$_\uparrow$ & LPIPS$_{\mathrm{(VGG)}\downarrow}$ \\
    \hline \hline
    
    8  & 4.8h & 24.44 & 0.687 & 0.432 \\
    16  & 4.9h & 25.05 & 0.712 & 0.401 \\
    32 & 5.1h & 26.16 & 0.748 & 0.379 \\ 
    \textbf{64}  & 5.5h & \textbf{26.83} & \textbf{0.769} & \textbf{0.364} \\
    128 & 6.3h & 25.73 & 0.721 & 0.385 \\ 
    
    \bottomrule
  \end{tabular}
  }
  \vspace{5ex}
  \centering
  \caption{\textbf{Impact of each components of attention mechanism.} We gradually incorporate scaling operations and position embeddings ($PE$) into the cross-resolution attention, while removing the Softmax operation from the pipeline. This is done to elucidate their roles in the global-local encoder, as discussed in \S \ref{sec:encoder}.}
  \label{tab:attention_mechanism}
  \scalebox{0.70}{
  % \begin{tabular}{@{}lcccc@{}}
  \begin{tabular}{l|ccc}
    \hline \thickhline
    \rowcolor{mygray}
    Attention  & PSNR$_\uparrow$ & SSIM$_\uparrow$ & LPIPS$_{\mathrm{(VGG)}\downarrow}$ \\
    \hline \hline
    
    Dot-Product    & 23.15 & 0.692 & 0.421 \\
    \midrule   
    + $\frac{1}{\sqrt{d_K}}$   & 24.36 & 0.728 & 0.398 \\
    + $\frac{1}{\sqrt{d_K}}$ + Softmax & 25.43 & 0.745 & 0.380 \\
    \textbf{+ $\frac{1}{\sqrt{d_K}}$ + Softmax + $PE$}  & \textbf{26.83} & \textbf{0.769} & \textbf{0.364} \\
    
    \bottomrule
  \end{tabular}
  }
  \end{minipage}
\end{table}

\section{Additional Implementation Details} 
\label{sec:add_implementation}

In \S \ref{sec:space_estimation}, the boundary factor for volume space estimation is held constant at $(0.5, 2.0)$, and the split distance threshold is fixed at $1.5$ during block subdivision, with a maximum octree intersection limit of 1024. The subdivision milestones are defined as $[2000, 4000, 6000, 8000, 10000]$, and the maximum allowed subdivision level is set to $16$. When constructing the global feature pool with a compact frequency of $1000$, the ray march fineness is calculated using the formula $e^{(i+\beta_0)(1-i)}$, where the initial fineness is initialized to $\beta_0=16$, and the fineness decay concludes at $10000$ iterations. For cross-resolution attention in \S \ref{sec:encoder}, we consider $10$ different resolution levels for a global-local scene representation, and the global-local encoder output dimension is 16. To guide the model using the proposed loss function in \S \ref{sec:loss}, a gradient scaling mechanism is employed, commencing at 1000 iterations and concluding at 5000 iterations. 
% As shown in Fig.~\ref{fig:more_disparity_loss}, the low-resolution disparity adopts reconstruction results from the first octree level, visibly revealing blocks that are positioned inaccurately but exhibit relative transparency.

\section{Additional Experiment Results}
\label{sec:add_exp}

We present additional qualification and quantification results based on our UAV datasets to facilitate a more comprehensive ablation study.

\subsection{Reality Capture \textit{v.s.} FPV-NeRF}
While 3D reconstruction tools like Reality Capture can explicitly generate a visible RGB model of a scene, the details often fall short when zoomed in, impeding the production of high-quality videos. Our method excels in rendering finer, more realistic details at a higher resolution than conventional 3D reconstruction techniques. For instance, as depicted in Fig.~\ref{fig:comparison_rc}, Reality Capture faces challenges in accurately rendering leaves, whereas our FPV-NeRF faithfully depicts each individual leaf.

\subsection{Impact of Block Subdivision Levels}
In \S \ref{sec:space_estimation}, we propose to subdivide the camera space into blocks and discuss the effectiveness of this operation in \S \ref{sec:ablation_study}. Here, we provide more details about the impact of the number of block subdivision levels. As illustrated in Table \ref{tab:subdivision_level}, an increase in the maximum division level enhances the rendering effect of the model. Optimal performance is achieved when employing a subdivision of 16 levels.

\subsection{Impact of Cross-Resolution Levels}
In \S \ref{sec:encoder}, we present a cross-resolution attention mechanism, showcasing its ability to improve both the overall structure and local detail in rendering results (as discussed in \S \ref{sec:ablation_study}). In this section, we explore the details of how the number of resolution levels in cross-attention affects our approach. As indicated in Table~\ref{tab:resolution_level}, increasing the number of resolution levels leads to improved rendering performance. This reinforces the significance of adopting cross-resolution attention across a broader range of resolutions.

\subsection{Effect of Attention Mechanism}
To compute the attention mechanism over different resolution with position embedding and scaled dot-product in \S \ref{sec:encoder}. In this section, we design ablation experiments to study the effectiveness of those components of attention mechanism. 
As indicated in Table~\ref{tab:attention_mechanism}, utilizing only the dot-product without scaling and position embedding yields the poorest performance. Introducing scaling with a factor of $\frac{1}{\sqrt{d_K}}$ improves rendering performance by 1.21 PSNR. Adding Softmax further enhances it by 1.07 PSNR, and incorporating position embedding results in a further improvement of 1.40 PSNR.

\subsection{Impact of Location Embedding Parameter}
We present additional comparison results for point location embedding, as illustrated in Fig.~\ref{fig:more_point_location}. By incorporating a higher number of sine and cosine frequency variations in Eq.~\ref{eq:point}, both the low-frequency and high-frequency component counts for point location embedding are increased, resulting in a clearer rendered first-person view video.

\subsection{Impact of MLP Dimension}
In \S \ref{sec:encoder}, the attention mechanism introduces numerous parameters. We aim to determine the optimal MLP dimension for the feature encoder and decoder, as evident in Fig.~\ref{tab:mlp_dim}. Both low and high dimensions yield suboptimal performance, emphasizing the need for a balanced parameter count. Experiments show that, with the attention mechanism's ample parameters, an MLP internal dimension of 64 suffices. Too few parameters hinder scene representation, while excessive ones may lead to overfitting on training frames, hindering the achievement of high-quality reconstruction.

\subsection{More Comparison Results With SOTA}
In \S \ref{sec:comparison_sota}, we demonstrate that FPV-NeRF surpasses previous SOTA methods in both quantitative and qualitative results. In this section, we present additional quantitative results for FPV-NeRF compared to previous SOTA methods, particularly at three different scales. As illustrated in Fig.~\ref{fig:more_comparison_sota}, FPV-NeRF outperforms previous SOTA methods at far, middle, and nearby distances, providing further evidence of its global-local perception capabilities.

% % 
% Having the supplementary compiled together with the main paper means that:
% % 
% \begin{itemize}
% \item The supplementary can back-reference sections of the main paper, for example, we can refer to \cref{sec:intro};
% \item The main paper can forward reference sub-sections within the supplementary explicitly (e.g. referring to a particular experiment); 
% \item When submitted to arXiv, the supplementary will already included at the end of the paper.
% \end{itemize}
% % 
% To split the supplementary pages from the main paper, you can use \href{https://support.apple.com/en-ca/guide/preview/prvw11793/mac#:~:text=Delete%20a%20page%20from%20a,or%20choose%20Edit%20%3E%20Delete).}{Preview (on macOS)}, \href{https://www.adobe.com/acrobat/how-to/delete-pages-from-pdf.html#:~:text=Choose%20%E2%80%9CTools%E2%80%9D%20%3E%20%E2%80%9COrganize,or%20pages%20from%20the%20file.}{Adobe Acrobat} (on all OSs), as well as \href{https://superuser.com/questions/517986/is-it-possible-to-delete-some-pages-of-a-pdf-document}{command line tools}.
